# Supplementary material for: Compact Parallel Hash Tables on the GPU
Source: arXiv:2406.09255 ancillary file (2024-06-13)
Supplement: Supplementary file 1 [file OVERVIEW.pdf]

# Compact Parallel Hash Tables on the GPU

## Artifact Overview

Steef Hegeman      Daan Wöltgens      Anton Wijs  
Alfons Laarman

May 15, 2024

This artifact supports the article “Compact Parallel Hash Tables on the GPU”, to appear in Euro-Par 2024. It consists of a basic header-only CUDA C++ library for compact cuckoo and compact iceberg hash tables, as well as benchmarks.

The file README.md contains information about the artifact as a compact GPU hash table library. There is a minimal example in the **examples** folder for host-side use, and the tests and comments included in the header files in **include** serve as further documentation.<sup>1</sup> The library can be used from the host and from the device side.

The rest of this document details how to verify the results in the aforementioned article, running the benchmarks and generating figures. It is also available in plain-text markdown (ARTIFACT.md), which might be useful for copying commands or referencing this document from a terminal environment.

## Getting Started Guide

### Hardware requirements

- A recent CUDA GPU with compute capability  $\geq 7.5$ 
  - The figures in the manuscript were generated on the RTX 4090. We have found comparable results on the RTX 3090 and NVIDIA L40s, but not on the older RTX 2080 Ti (where compactness gives only a slight performance benefit.)
  - Some results are only achieved at high load. For this reason, benchmarks can be completed faster on GPUs with smaller memory. (For verification, a high-end GPU such as the L40s may thus not be desirable.)
- Roughly as much RAM as the GPU has memory
- Roughly as much free storage space as the GPU has memory

---

<sup>1</sup>The **doctest** tests are ignored during normal compilation. They can also be stripped from the headers if desired.

## Software requirements

- A relatively up-to-date Linux distribution
- Version 12 of the CUDA Toolkit, preferably 12.4, and matching drivers
  - The toolkit can be obtained at <https://developer.nvidia.com/cuda-toolkit>
- Python 3 and the ability to create virtual environments (venv / pip)
  - On some systems, the latter may require an extra package (`python3-venv` on Ubuntu)
  - The minimal Python version we tested is 3.7.13, but newer is recommended.
- For the real-world benchmark, `xz` is required to decompress the data.
- As the project uses C++20 features, a relatively recent compiler is required. We used `g++ 11.0.4`.

The library itself depends only on the CUDA toolkit and can be used by simply copying over the files in the `include` directory. The additional requirements are for running the benchmarks and producing the figures.

## Setting up

1. Open a shell at the root directory of the artifact
2. Create and activate a Python virtual environment, and install dependencies:

```
python3 -m venv venv
source venv/bin/activate
pip install -r python-requirements.txt
```

This installs specific versions of the Python dependencies for compilation (`meson`, `ninja`), and the benchmark data / figure generation (`numpy`, `pandas`, `tomli`, and `matplotlib`) in the local virtual environment. If the install command raises an error (which may happen for older Python versions like Python 3.7), a working environment can likely be created with

```
pip install meson ninja numpy pandas tomli matplotlib
```

When launching a new shell, the virtual environment should again be activated.

3. Compile the project in release mode

```
meson setup release --buildtype=release -Dwerror=false
meson compile -C release
```

`meson` will automatically download specific versions of the C++ dependencies: `doctest` for the tests, `argparse` and `nlohmann-json` for command line argument and JSON parsing in the benchmark runners. (Though we will not use JSON here.)

4. Run the tests with

```
./release/tests
```

They should all pass.

We are now ready to run the benchmarks.

## Step-by-step instructions

### Main benchmarks

For convenience, a benchmark suite and figure generation can be performed with

```
./benchmarks/benchmarks.sh SIZE
```

where **SIZE** is one of: **micro**, **tiny**, **small**, **normal**, **large**. The benchmark results will only be representative if the system is put under load, so it is important to choose the right benchmark size for the GPU. The **small** benchmark is suitable for GPUs with around 12GB of memory, the **normal** benchmark for those with 24GB of memory, and the **large** one for those with 48GB of memory. The **tiny** benchmark can be used to quickly verify that the benchmark process works. The others may take one or more hours (see below).

**Results** After the script is finished, the **out-SIZE** directory contains pdf files of figures corresponding to those in the manuscript. For comparison, the manuscript figures can be found in the **reference** directory.

**Runtime** The **tiny** benchmark, though not at all representative for a system under load, should complete in less than half an hour (less than a minute on our RTX 4090). The **normal** benchmark takes roughly 30 minutes on an RTX 4090.

### Real-world (havi) benchmark

The real-world benchmark that appears in the article can be performed with

```
./benchmarks/benchmarks.sh havi
```

and should complete within 5 minutes. The output can be found in **out-havi**.

The input data is included with the artifact in the file **havi-log.txt.xz**. The benchmark script will decompress this and convert it to a binary file **havi.bin** before passing it to the **./release/havi** benchmark runner.

### Reference output

The **reference** directory contains the benchmark results used for the manuscript and generated figures for comparison. These results were generated on an RTX 4090 with 24GB memory with a benchmark setup comparable to the **normal** parameters. (See below for a more accurate description.) The host machine had an Intel Xeon Silver 4214R processor and 240GB of RAM.

## Research notes and troubleshooting

### My GPU has much less than 12GB (or much more than 48GB) of memory

The `benchmarks.sh` script can also be supplied with an integer, in which case this will be taken as the logarithm of the number of (primary) entries in the benchmark tables. The `normal` size for GPUs with 24GB memory corresponds to the integer 27, and each step roughly halves or doubles the memory used. For GPUs with 6GB of memory one may try `./benchmarks/benchmarks.sh 25`.

### Fine-grained benchmarks

For further research, it may be useful to run more fine-grained benchmarks. The interested reader may inspect the `--help` output of `release/rates`, `benchmarks/generate.py` and `benchmarks/figures.py`.

### Increasing the precision

Apart from increasing the benchmark size, precision may also be improved by taking more measurements. A measurement consists of many table benchmarks, each consisting of multiple runs. Measurements correspond with taking new random variables (for the permutations). We have not observed much variance between measurements, but confidence increases with the number of measurements. The number of runs per measurement corresponds with running the same setup multiple times (of which the first is always discarded as warmup).

The figures in the manuscript were generated on an RTX 4090 with 10 measurements, each measurement consisting of 3 runs per benchmark.

The number of measurements can be controlled via the `N_MEASUREMENTS` variable in `benchmark/benchmarks.sh` (via a command-line argument to the `rates` benchmark runner). The `N_RUNS` constant in `benchmarks/benchmarks.cu` can be used to control the number of runs (and the project needs to be recompiled afterwards with `meson compile -C release`). The exact same benchmark as run on our RTX 4090 for the manuscript can be performed with

```
./benchmarks/benchmarks.sh manuscript
```

### A note on unified memory

With unified (managed) memory (which in particular automatically swaps GPU memory to the CPU RAM), larger table sizes can be benchmarked. Here, we have found the compact tables to greatly outperform non-compact tables, likely because the non-compact tables have to swap more. As this is thus not a fair comparison, we have removed this from our benchmarks. All relevant allocations can however be forced to use managed memory by editing `include/cuda_util.cuh`, replacing the contents of the `alloc_dev` function with that of `alloc_man` in the

same file. After a recompilation, larger benchmark sizes can be run, though a whole benchmark will take several hours.
